# Supplementary material for: Magnetic ordering and structural phase transitions in strained ultrathin SrRuO$_{3}$/SrTiO$_{3}$ superlattice
Source: arXiv:1208.5945 source file (2012-08-29)
Supplement: Supplementary file 1 [file sup_mat_0701.pdf]

# Supplementary Materials for the manuscript "Magnetic ordering and structural phase transitions in strained ultrathin $SrRuO_3/SrTiO_3$ superlattice"

Mingqiang Gu,[1,2] Qiyun Xie,[1] Xuan Shen,[4]
Rubin Xie,[1] Jianli Wang,[3] Gang Tang,[3] Di Wu,[4] G. P. Zhang,[2] and X. S. Wu[1*]

[1]*Laboratory of Solid State Microstructures and School of Physics, Nanjing University, Nanjing 210093, China*

[2]*Department of Physics, Indiana State University, Terre Haute, IN 47809*

[3]*Department of Physics, China University of Mining and Technology, Xuzhou 221116, China*

[4]*Laboratory of Solid State Microstructures and Department of Materials Science and Engineering, Nanjing University, Nanjing 210093, China*

* Corresponding author: xswu@nju.edu.cn

These supplementary materials include the experimental setup to grow and characterize three $SrRuO_3/SrTiO_3$ superlattice samples, the detail of our first-principles calculations, the role of the Hubbard U, and the evolution of the electronic structures.

## A. Experimental setup

Three superlattice samples with 30 [SRO/STO] periods were fabricated on a) STO, b) Nb:STO, and c) LaSrAlTaO (LSAT) substrates. The in-plane lattice constants for the substrates are 3.905 Å, 3.907 Å and 7.738 Å (effectively 3.869 Å), respectively. In other words, the lattice mismatches for these substrates are 0%, 0.05% and -0.92% (in terms of STO lattice constant), respectively. Superlattices were grown using laser-MBE at 750 °C, with the repetition frequency (2 Hz) and the constant laser intensity of 60 mJ/3.4 $mm^2$. All the samples were grown under an oxygen pressure of 0.005 mbar. Reflection high energy electron diffraction (RHEED) was used to monitor the entire growth process. A layer-by-layer growth mode was found. From the RHEED pattern, the period for the SRO/STO superlattice is recognized as 1/1. Atomic force microscopy was used to probe the roughness of these samples, which shows very smooth terminations with the surface roughness less than 1 uc, see Fig. S1.

The samples were characterized by means of x-ray diffraction data (shown in Fig. S2) collected at the Rigaku DmaxrB diffractometer (wavelength $\lambda = 1.54$ Å) as well as the beamline BL14B1 of Shanghai Synchrotron Radiation Facility ($\lambda = 0.688$ Å), at room temperature. BL14B1 is a beamline based on bending magnet and a Si(1 1 1) double crystal monochromator was employed to monochromatize the beam. The size of the focus spot is about 0.5 mm and the end station is equipped with a Huber 5021 diffractometer. NaI scintillation detector was used for data collection. The (001) and (002) peaks in Fig. S2 clearly show that the samples have an orientation parallel to $c$ axis. The total thicknesses of the superlattices calculated from the distance between interference stripes are 212 Å, 233 Å and 210 Å, respectively. The glazing incident X-ray reflection measurements by synchrotron radiation (with the wavelength of 0.1238 nm) were performed. The $(00\frac{1}{2})$ peak (Fig. S2(c)) at $\sim 9^\circ$ shows the 1/1 periodicity of our samples.

### B. Details of the DFT calculation

First-principles calculations are performed using the Vienna ab-initio Simulation Package (VASP) [1]. An in-plane $\sqrt{2} \times \sqrt{2}$ tetragonal geometry is adopted to allow the rotation of the octahedra, with its in-plane lattice constants confined to reflect the strain. We use a plane-wave cutoff energy of 500 eV and the $(6 \times 6 \times 6)$ Monkhorst-Pack $k$-point mesh to converge the total energy within 0.01 eV. Inversion symmetry is kept during the structural optimization. The correlation effect of Ru-4$d$ electrons is taken into account with $U$ = 2.5 eV and $J$ = 0.4 eV, within the Dudarev *et al.*'s scheme [2]. The values of $U$ and $J$ are consistent with previous studies [3], giving a reliable description to our system. For strain-free bulk materials, the calculated lattice constants ($a$=$b$=$c$=3.865 Å for STO, and $a$=5.517, $b$=5.502, $c$=7.775 Å for SRO) are in good agreement with the experiment values [4, 5] and prior DFT studies [6, 7].

The contribution of carriers to the optical properties in the metallic phase includes both intraband and interband transitions. After the structure optimizations are done with VASP, the optical properties for these optimized structures are calculated with the Wien2K code [8], since VASP does not include the intraband contribution. The k-point convergence in the optical calculation should be treated carefully, especially for metal [9]. In our work, the k-point convergence has been tested (see Fig. S3) and increased to $(14 \times 14 \times 10)$ in the first Brillouin Zone. The optical dielectric tensor is then calculated from

$$\varepsilon(\mathbf{q} \to 0, \omega) = 1 + \varepsilon^{\{intra\}}(\mathbf{q} \to 0, \omega) + \varepsilon^{\{inter\}}(\mathbf{q} \to 0, \omega), \tag{1}$$

where $\varepsilon^{\{intra\}}$ and $\varepsilon^{\{inter\}}$ are intraband and interband contributions, respectively. The intraband transition is included as a correction for low energy transitions by simply adopting the Drude model:

$$\mathrm{Im}\varepsilon_{ij}^{\{intra\}}(\omega) = \frac{\Gamma \omega_{\mathrm{p}ij}^2 \delta_{ij}}{\omega(\omega^2 + \Gamma^2)} \tag{2}$$

where $\omega_\mathrm{p}$ is the plasma frequency for metallic phase, and $\Gamma$ is the life-time broadening. $\omega_\mathrm{p}$ is determined by the carrier concentration and effective mass of the conduction electron. We take the reported bulk data [10] from Hall measurement ($\omega_\mathrm{p}$ = 30517 cm$^{-1}$ $\approx$ 3.78 eV, $\Gamma$ = 0.8 eV). The $\delta$ function here ensures the intraband contribution for the off-diagonal element to be zero [11]. The interband contribution is calculated as

$$\varepsilon^{\{inter\}}(\omega) = -\frac{4\pi\hbar^2 e^2}{\Omega m_e^2} \lim_{\mathbf{q}\to 0} \sum_{c,v,\mathbf{k}} \frac{(\mathbf{p}_{c,v,\mathbf{k}} \cdot \mathbf{q}/|\mathbf{q}|)^2}{(\epsilon_{c,\mathbf{k}} - \epsilon_{v,\mathbf{k}} - \omega)(\epsilon_{c,\mathbf{k}} - \epsilon_{v,\mathbf{k}})^2} \quad (3)$$

where $\Omega$ is the unit cell volume, $m_e$ the electron mass. $\mathbf{p}_{c,v,\mathbf{k}}$ is the momentum matrix element between the conduction state $c$ and valence state $v$ with crystal momentum $\mathbf{k}$. $\mathbf{q}$ denotes the Bloch vector of the incident wave. $\epsilon_{c\mathbf{k}}$ and $\epsilon_{v\mathbf{k}}$ are respectively conduction and valence band energies at wave vector $\mathbf{k}$.

### C. The choice of $U$ and its role on our results

To describe the correlation effects of strontium ruthenate properly, effective on-site Coulomb repulsion ($U_{\text{eff}} = U - J$) is always taken into account. In previous studies the value of $U_{\text{eff}}$ ranges from 0 eV to 4 eV [3, 12–15]. Due to the screening effects of the extended 4d electrons, the on-site correlation is less important than that in 3d transition metal oxides such as manganites or ferrites. In our present work, we selected a modest value, i.e. $U_{\text{eff}} = 2.1$ eV, similar to that by Mahadevan *et al* [3].

In comparison with our experiments, our theoretical results with $U_{\text{eff}} = 2.1$ eV overestimate the magnetization. The magnetization from experiment ranges from $0.12 \pm 0.03$ $\mu_B$ to $0.30 \pm 0.03$ $\mu_B$, while that from LSDA+U is always 2 $\mu_B$. This is because the Hubbard U increases the splitting of Ru spins, making it fully saturated. Rondinelli *et al.* [13] showed that a similar choice of U ($U_{\text{eff}} > 1.6$ eV) always leads to such a half-metallic state. The deviation between theory and experiment may be due to two reasons: The supercell in our theory is infinite large while experimentally there are only 30 periods in the thin films; the LSDA+U here is only approximately taking into account the correlation effects.

In order to see the strain effects on the magnetic moment, we set $U_{\text{eff}}$ to 0 eV and investigate the change of magnetic moment as a function of strain. The result is plotted in the inset of Fig. 1(b). It clearly shows that the trend of the magnetic moment change is consistent with the experimental results. The agreement between theory and experiment validates the use of DFT method to investigate the properties for this system.

We find the choice of $U_{\text{eff}}$ does not have drastic impacts on the crystal structure. Table S1 shows a maximum 9% change found in $\theta_{\text{Ru}}$. More importantly, the first structural phase transition exists regardless of the value of $U_{\text{eff}}$. This shows the robustness of our result. Our result is also consistent with prior phase transitions in bulk SRO and other perovskites

observed experimentally [17–19]. Even though the rotation angles do not vary a lot, the $\alpha \rightarrow \beta$ phase boundary for the threshold of octahedra tilting depends on $U$ (shown in Fig. S4). This presents an opportunity to determine $U_{\text{eff}}$ by comparing our theoretical result with future experimental data.

The magnetic and electronic phase transition in the high strain region strongly depends on $U_{\text{eff}}$, since $U_{\text{eff}}$ is responsible for the insulating phase. Figure S5 shows that the plain LSDA calculation ($U_{\text{eff}} = 0$) predicts that the FM phase persists up to 8%, which is unrealistic from the results in the similar compounds [20]. This shows the crucial role of the electron correlation in this phase transition. We should emphasize that for the bulk SRO, however, with the same magnitude of U neither the A-type nor the C-type AFM configuration can not yield an insulating phase. Hence the superlattice configuration, i.e. the insertion of insulating STO layer between SRO layers, facilitates the metal-to-insulator transition. This will be discussed further in the next part.

### D. Evolution of the electronic structure vs strain

In order to get insight into the electronic structure that underlies these phase transitions, we examine the density of states (DOS) in Figs. S6 and S7. The transport property in this system is mainly dominated by SRO layer, specifically, the Ru-4$d$ orbital. The FM phase reserves the theoretical half-metallic ground state for bulk SRO. This ground state coincides with the ionic model: the $Ru^{4+}$ ion in the high spin state abeys Hund's rule, with the alignment of the four 4$d$ electrons as ($t_{2g}^3 \uparrow, t_{2g}^1 \downarrow$). The conducting states are composed of hybridized Ru-4$d$ and O-2$p$ orbitals while the Ti-3$d$ states are about 2 eV higher than the Fermi level. The conduction carriers are confined in the two dimensional SRO layer [15].

Tensile strain alters the electronic structures by changing the bond lengths. Increasing the in-plane lattice constant shortens the B-$O_{\text{apex}}$ bond and elongates the B-$O_{\text{in-plane}}$ bonds (Table S2). This changes the projected density of states and band structures (shown in Fig. S7). When strain is small, the octahedral distortion and the chemical modulation along the $z$-axis lift the degeneracy of $t_{2g}$ orbitals. This results in a narrower $d_{xy}$ band and broader $d_{yz/zx}$ doublet. As strain increases, the band width of spin-up $d_{xy}$ is broadened, at the same time the energy of $d_{yz/zx}$ bands is lowered. This reduces the $t_{2g}$ splitting, and changes the occupation of spin-down electrons for these orbitals given in Fig. 2(b) in the main text and

Fig. S8.

Further increasing the strain leads to the metal-to-insulator transition. As mentioned above, the superlattice configuration facilitates this transition with the confinement of the extended 4d states along the $z$ direction. The transition depends on the ratio of the on-site Coulomb interaction with respect to the hopping integral, i.e. $U/t$ [21]. The electron hopping between the neighboring $d_{\mathrm{yz/zx}}$ orbitals is blocked due to the quantum confinement effect at interface [22], leaving only that among the $d_{\mathrm{xy}}$ orbitals. As the in-plane strain increased, the overlap of $d_{\mathrm{xy}}$ orbitals is reduced. The hopping integral between neighboring Ru atoms becomes smaller. At the critical point, a sharp change in occupation of these orbitals then occurs. This is the sign of the metal-to-insulator transition. In the AFM phase, one minority electron is mostly in the $d_{\mathrm{xy}}$ orbital, leaving the $d_{\mathrm{yz/zx}}$ unoccupied. Thus this phase transition is orbital-selective. The narrow subband features near the Fermi energy in Fig. S7 show that both the $d_{\mathrm{xy}}$ and the $d_{\mathrm{yz/zx}}$ doublet bands are highly confined in this phase.

---


[1] G. Kresse and J. Furthmüller, Computational Materials Science **6**, 15 (1996).

[2] S. L. Dudarev, G. A. Botton, S. Y. Savrasov, C. J. Humphreys and A. P. Sutton, Phys. Rev. B **57**, 1505 (1998).

[3] P. Mahadevan, F. Aryasetiawan, A. Janotti and T. Sasaki, Phys. Rev. B **80**, 035106 (2009).

[4] O. Nakagawara, M. Kobayashi, Y. Yoshino, Y. Katayama, H. Tabata and T. Kawai, J Appl. Phys. **78**, 7226 (1995).

[5] C. W. Jones, P. D. Battle, P. Lightfoot and W. T. A. Harrison, Acta Crystallogr. Section C **45**, 365 (1989).

[6] M. Gu, J. Wang, Q. Y. Xie and X. S. Wu, Phys. Rev. B **82**, 134102 (2010).

[7] A. T. Zayak, X. Huang, J. B. Neaton and K. M. Rabe, Phys. Rev. B **74**, 094104 (2006).

[8] C. Ambrosch-Draxl and J. O. Sofo, Computer Physics Communications **175**, 1 (2006).

[9] G. P. Zhang, Y. Bai and T. F. George, Physical Review B **80**, 214415 (2009).

[10] M. H. Kim, G. Acbas, M. H. Yang, M. Eginligil, P. Khalifah, I. Ohkubo, H. Christen, D. Mandrus, Z. Fang and J. Cerne, Phys. Rev. B **81**, 235218 (2010).

[11] P.M. Oppeneer, *Magneto-optical Kerr Spectra*, in *Handbook of Magnetic Materials, Vol. 13*, edited by K.H.J. Buschow (Elsevier, Holland, 2001)

[12] A. T. Zayak, X. Huang, J. B. Neaton and K. M. Rabe, Phys. Rev. B **77**, 214410 (2008).

[13] J. M. Rondinelli, N. M. Caffrey, S. Sanvito and N. A. Spaldin, Phys. Rev. B **78**, 155107 (2008).

[14] H.-T. Jeng, S.-H. Lin and C.-S. Hsue, Phys. Rev. Lett. **97**, 067002 (2006).

[15] M. Verissimo-Alves, P. García-Fernández, D. I. Bilc, P. Ghosez, J. Junquera, Phys. Rev. Lett. **108**, 107003 (2012).

[16] L. de Medici, J. Mravlje and A. Georges, Phys. Rev. Lett. **107**, 256401 (2011).

[17] A. Y. Borisevich, H. J. Chang, M. Huijben, M. P. Oxley, S. Okamoto, M. K. Niranjan, J. D. Burton, E. Y. Tsymbal, Y. H. Chu, P. Yu, R. Ramesh, S. V. Kalinin and S. J. Pennycook, Phys. Rev. Lett. **105**, 087204 (2010).

[18] A. Vailionis, H. Boschker, W. Siemons, E. P. Houwman, D. H. A. Blank, G. Rijnders and G. Koster, Phys. Rev. B **83**, 064101 (2011).

[19] J. He, A. Borisevich, S. V. Kalinin, S. J. Pennycook and S. T. Pantelides, Phys. Rev. Lett. **105**, 227203 (2010).

[20] G. Koster, L. Klein, W. Siemons, G. Rijnders, J. S. Dodge, C.-B. Eom, D. H. A. Blank and M. R. Beasley, Rev. Mod. Phys. **84**, 253 (2012).

[21] J. Hubbard, Proc. R. Soc. Lond. A **281**, 401 (1964).

[22] Y. J. Chang, C. H. Kim, S. H. Phark, Y. S. Kim, J. Yu and T. W. Noh, Phys. Rev. Lett. **103**, 057201 (2009).

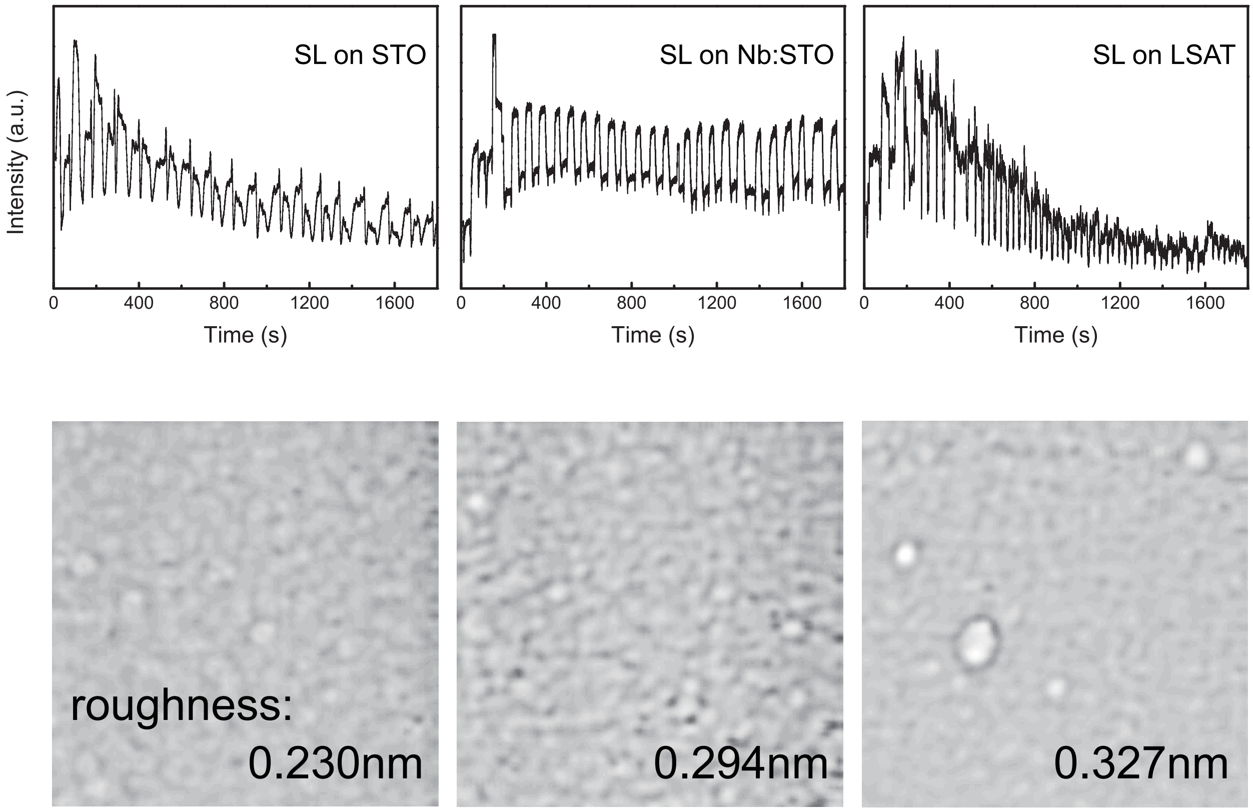


FIG. S1: (Color online) Upper panel: RHEED intensity during the growth of the superlattice samples as a function of time. Lower panel: Surface AFM image. Figures from left to right are for $[SRO/STO]_{30}$ superlattices grown on STO, Nb:STO, LSAT substrates, respectively. It shows a very smooth termination. The roughnesses are shown in the graph.

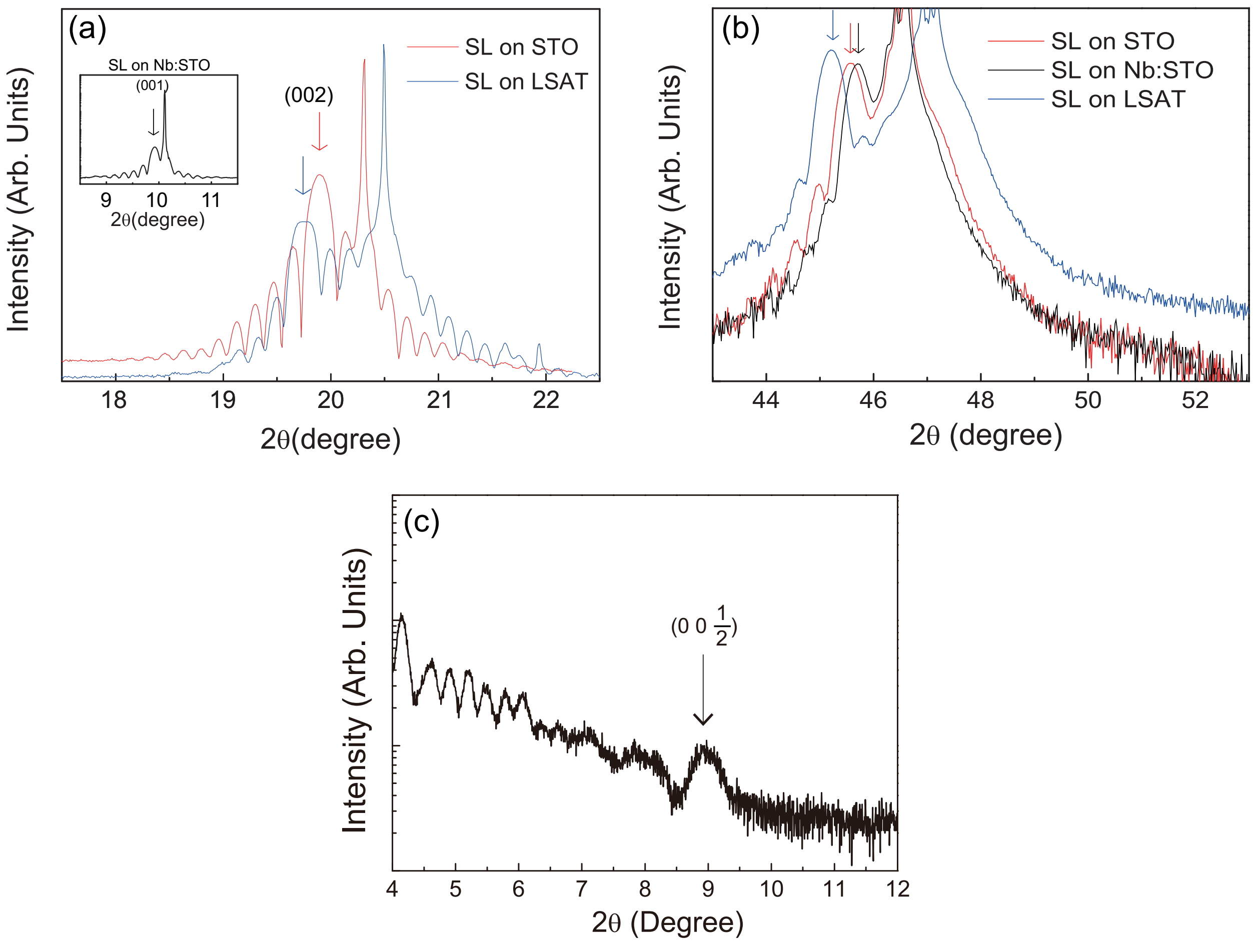


FIG. S2: (Color online) X-ray diffraction data collected from (a) synchrotron radiation and (b) Rigaku DmaxrB diffractometer. The (002) peaks for different samples are denoted. Inset in (a) shows the (001) peak. (c) The $(00\frac{1}{2})$ peak shows the 1/1 periodicity of the superlattice.

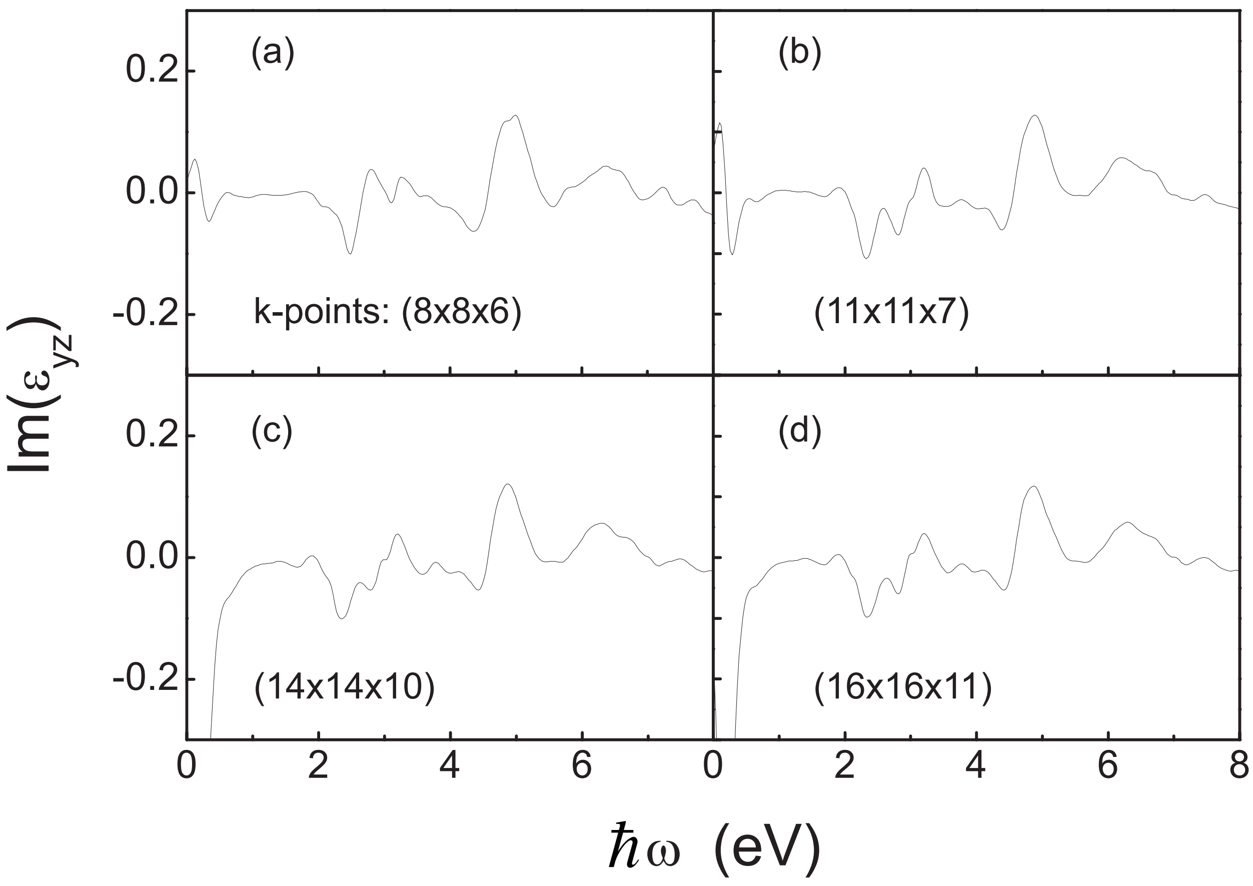


FIG. S3: K-point convergence of optical calculation for a fixed strain $\xi = 1\%$. The k-point mesh from (a) to (d) is $(8 \times 8 \times 6)$, $(11 \times 11 \times 7)$, $(14 \times 14 \times 10)$, $(16 \times 16 \times 11)$, respectively

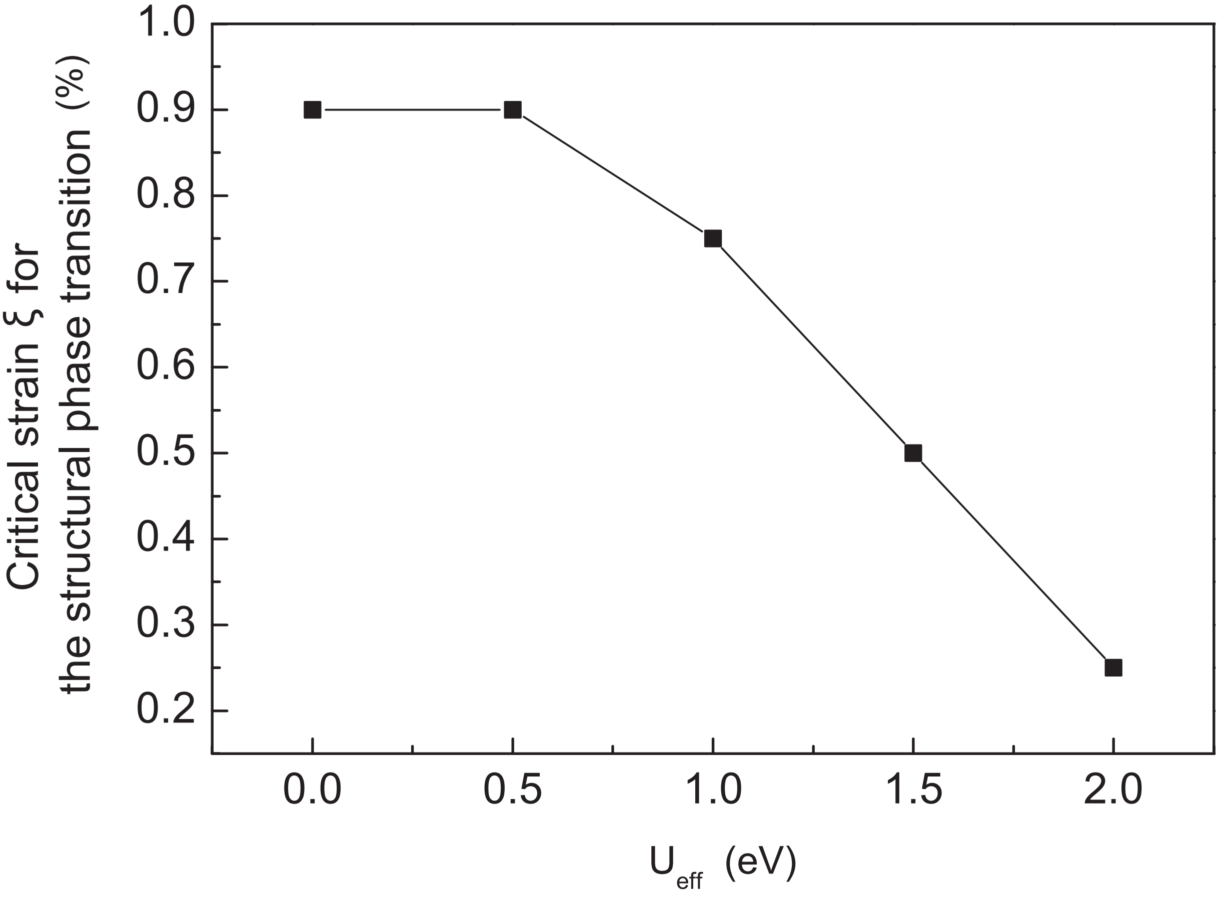


FIG. S4: The critical strain for the $\alpha$ to $\beta$ phase transition as a function of $U_{\rm eff}$.

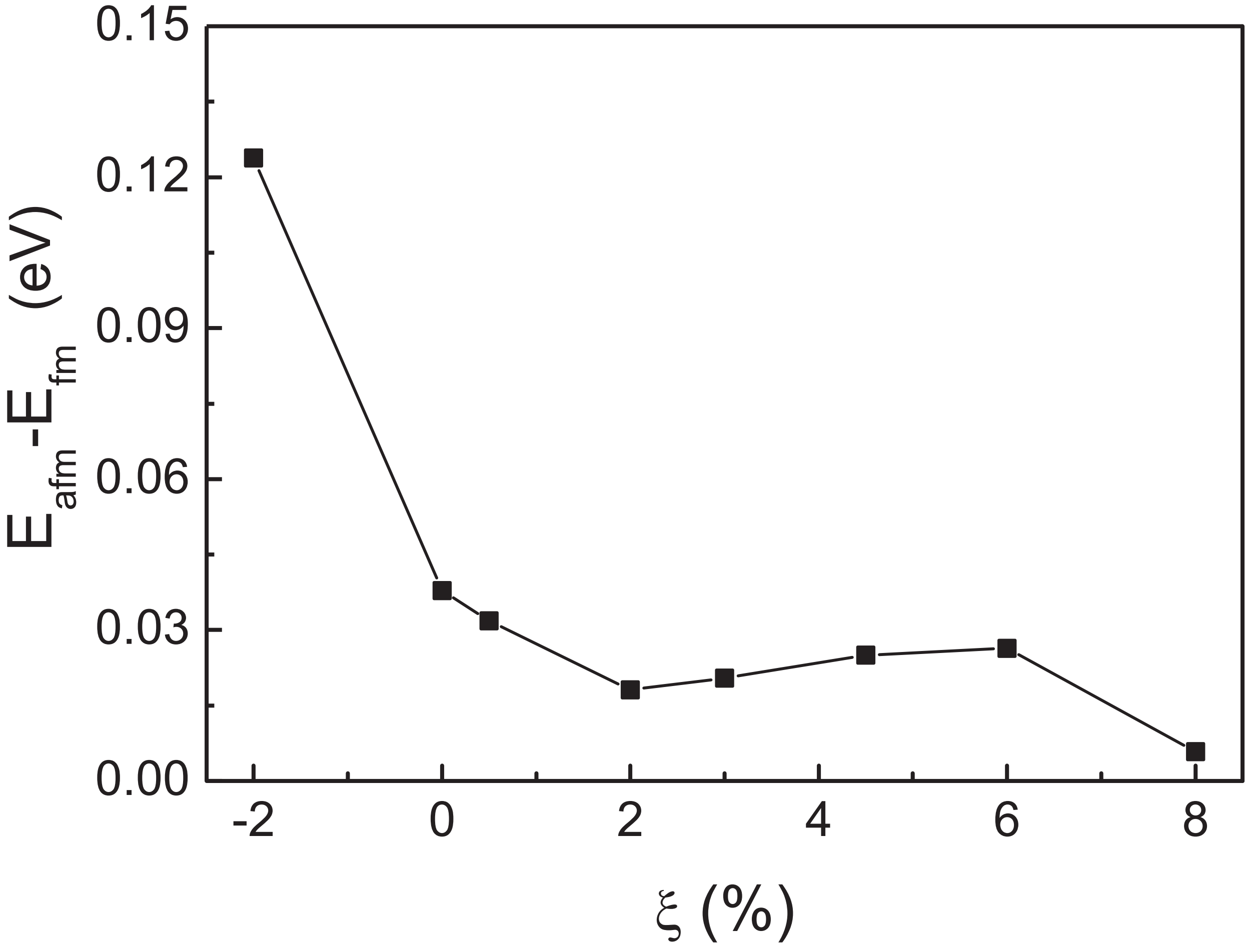


FIG. S5: Total energy difference between AFM and FM orderings as a function of strain in the plain LSDA calculation.

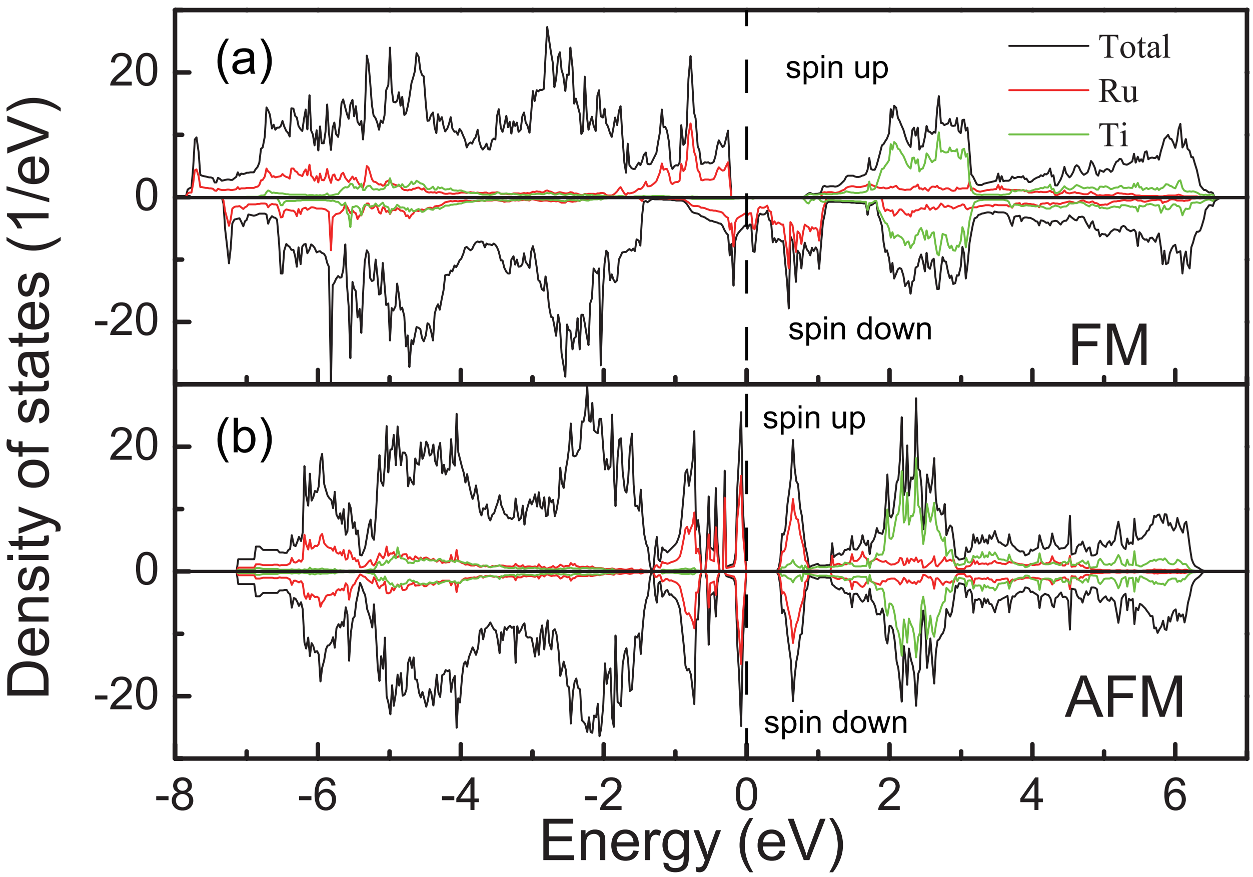


FIG. S6: (Color online) Total density of states. (a) and (b) show the DOS for the FM ($\xi = 1\%$) and AFM ($\xi = 5.5\%$) phases, respectively. Fermi energy is set to 0 eV. The red (green) line denotes the contributions from the Ru (Ti) atoms.

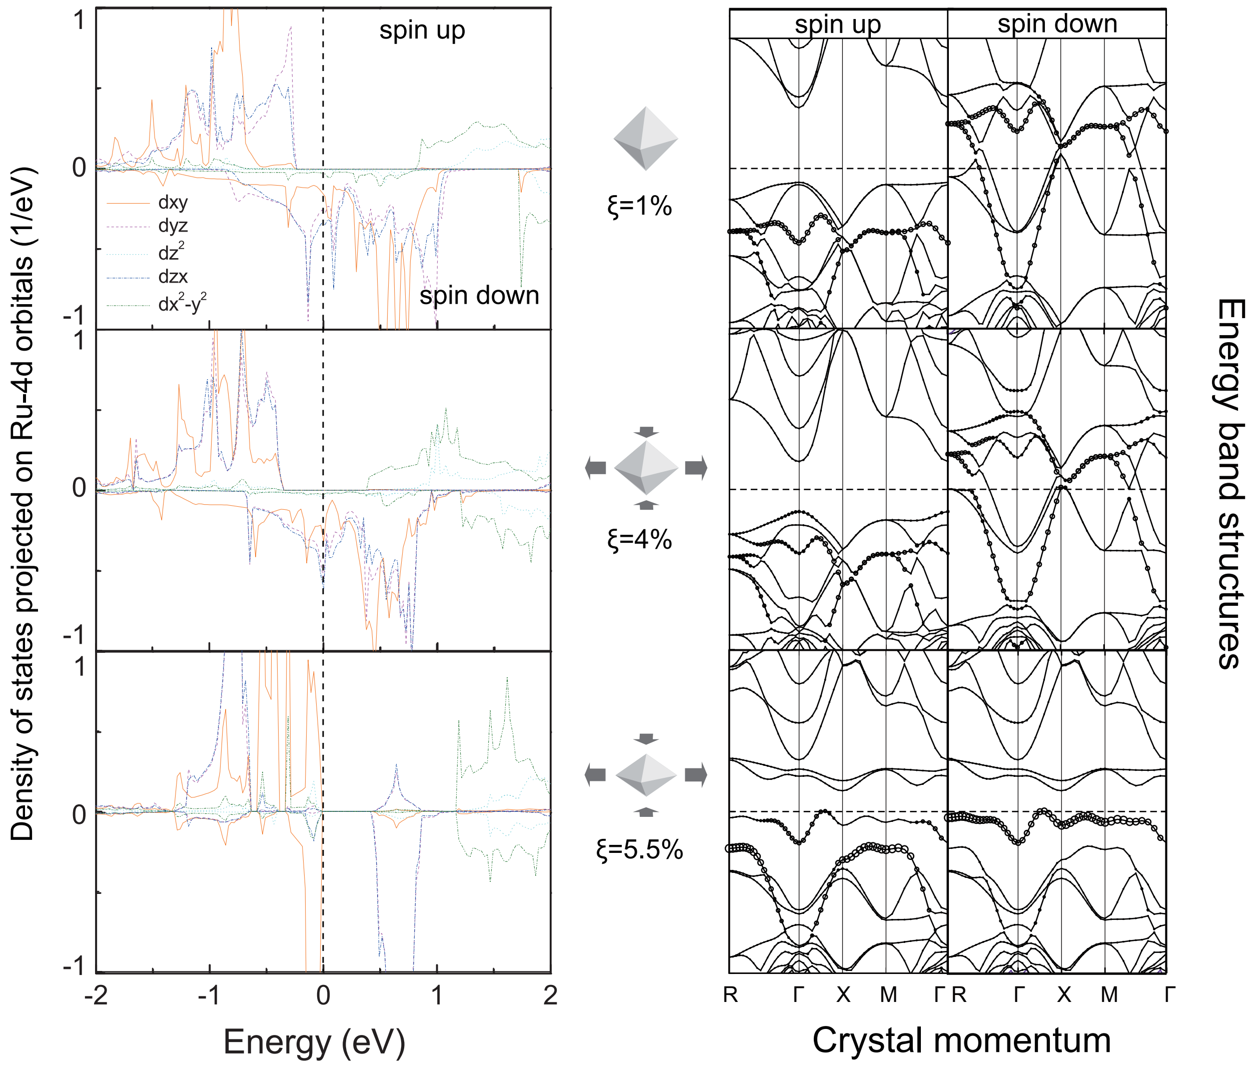


FIG. S7: (Color online) From top to bottom: $\xi = 1\%$, $\xi = 4\%$, $\xi = 5.5\%$. Left panel: Density of states projected on the Ru $4d$ orbitals. Right panel: Band structure of the superlattice at different strain. The dashed lines denote the Fermi level. The radii of circles in the band structure denote the weight of the $d_{\mathrm{xy}}$ electrons.

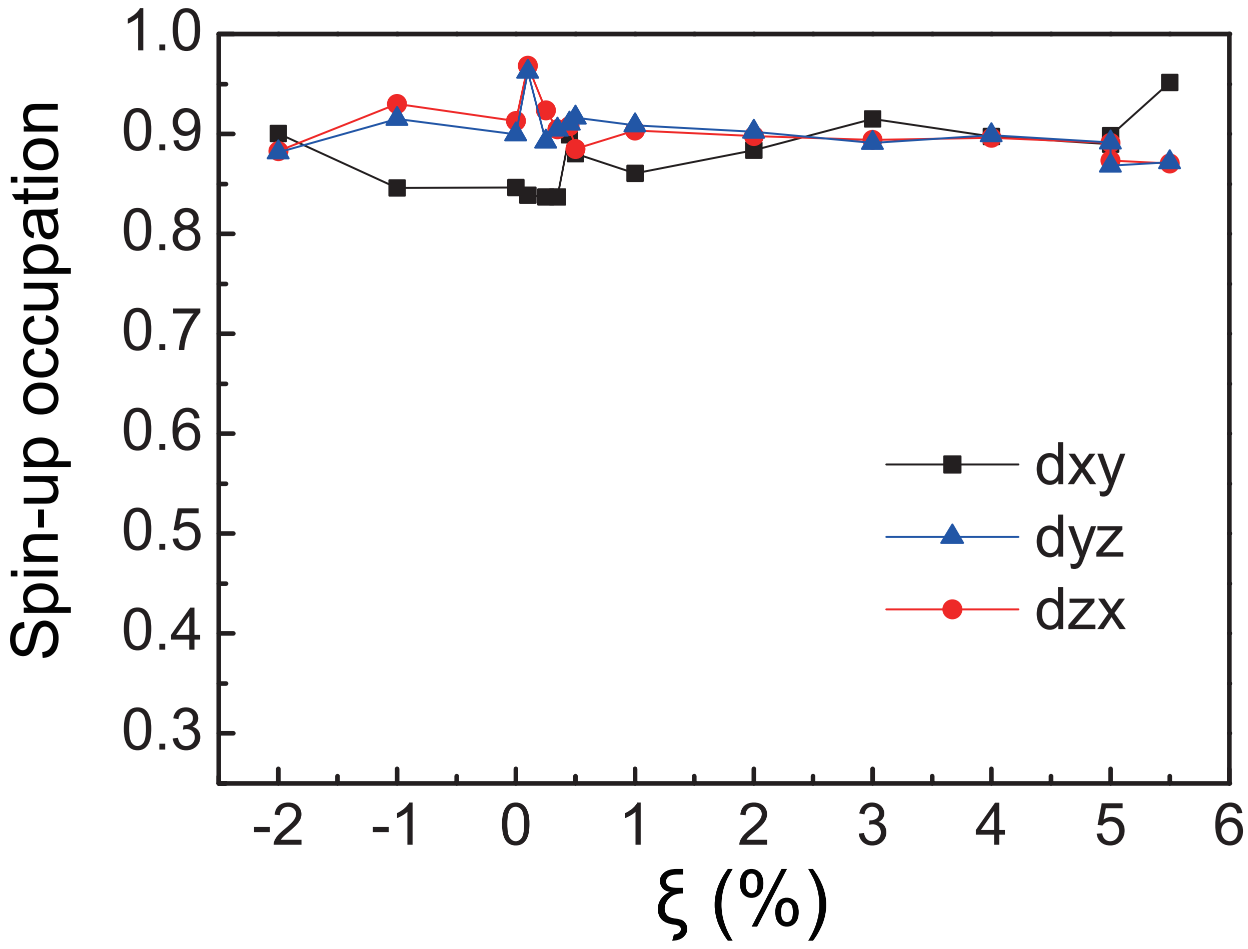


FIG. S8: (Color online) Spin-up occupation of the three $t_{2g}$ orbitals as a function of strain. In comparison to the spin-down channel shown in Fig. 2(b) of the main text, the spin-up channel shows a weaker dependence on the strain change.

TABLE S1: Comparison of tilting and rotation angles between the LSDA+U and plain LSDA calculations.

| | LSDA+U ($U_{eff}$=2.1 eV) | | | plain LSDA ($U_{eff}$=0 eV) | | |
|---|---|---|---|---|---|---|
| $\xi$ | $\phi$ (deg) | $\theta_{Ru}$ (deg) | $\theta_{Ti}$ (deg) | $\phi$ (deg) | $\theta_{Ru}$ (deg) | $\theta_{Ti}$ (deg) |
| -2% | 0 | 12.97 | -6.41 | 0 | 11.94 | -6.97 |
| 0% | 0 | 11.21 | -4.96 | 0 | 10.17 | -4.64 |
| 3% | 7.98 | 5.72 | 1.08 | 7.37 | 5.94 | 1.17 |

TABLE S2: Bond lengths in the $RuO_6$ and $TiO_6$ octahedra at different phases. Values in parenthesis are the corresponding strains.

| Phase ($\xi$ in %) | Ru-$O_{apex}$ (Å) | Ru-$O_{in\text{-}plane}$ (Å) | Ti-$O_{apex}$ (Å) | Ti-$O_{in\text{-}plane}$ (Å) |
|---|---|---|---|---|
| $\alpha$ (-1) | 1.996 | 1.956 | 1.934 | 1.922 |
| $\alpha$ (0) | 1.981 | 1.971 | 1.918 | 1.939 |
| $\beta$ (1) | 1.973 | 1.983 | 1.912 | 1.954 |
| $\gamma$ (4) | 1.945 | 2.029 | 1.888 | 2.018 |
| AFM (5.5) | 1.912 | 2.077 | 1.881 | 2.042 |
